# Supplementary material for: Hybrid Computing for Interactive Datacenter Applications
Source: arXiv:2304.04488 source file (2023-04-10)
Supplement: Supplementary file 1 [file appendix.tex]

\section{Appendix}
\label{sec:appendix}
